# Supplementary material for: Disordered BKT transition and superinsulation
Source: arXiv:1706.00555 ancillary file (2017-07-21)
Supplement: Supplementary file 1 [file si_VF.pdf]

# Supplementary Information: Criticality of the BKT transition and superinsulation

S. Sankar, V. Vinokur & V. Tripathi
*Department of Theoretical Physics, Tata Institute of Fundamental Research, Homi Bhabha Road, Navy Nagar, Mumbai 400005, India*
*Materials Science Division, Argonne National Laboratory, Argonne, Illinois 60439, USA.*

## A. Renormalization group analysis

In this section we show the essential steps followed for obtaining the phase diagram and critical behavior of the two-dimensional Coloumb gas under a logarithmically correlated quenched disorder potential . Inorder to account for the quenched disorder, a renormalization group (RG) approach using the replica method is adopted. A comprehensive study can be found in Ref. [1].

The partition function of the replicated Coulomb gas with *m-vector* charges after averaging over the bare disorder is

$$\overline{Z^m} = 1 + \sum_{p=2}^{\infty} \sum_{\mathbf{n}_1,\ldots,\mathbf{n}_p} \int_{|\mathbf{r}_i - \mathbf{r}_j| > a_0} \exp(-\beta H^{(m)}[\mathbf{n}, \mathbf{r}]),$$

where the sum is over all distinct neutral configurations and

$$\beta H^{(m)} = \sum_{i \neq j} K_{ab} n_i^a \ln\left(\frac{|\mathbf{r}_i - \mathbf{r}_j|}{a_0}\right) n_j^b + \sum_i \ln Y[\mathbf{n}_i].$$

Here, $Y[\mathbf{n}] = \exp(-n^a \gamma K_{ab} n^b)$, where $K_{ab} = \beta E_C \delta_{ab} - \eta \beta^2 E_C^2$. Significant contribution to the partition function only comes from charges $\pm 1, 0$ and hence we resctrict to these. We increase the hard core cutoff $a_0 \to a_0 e^{(d\ell)}$ and retain the original form of the partition function in terms of scale dependent coupling constants $(K_\ell)_{ab}$ and fugacities $Y_\ell[\mathbf{n}]$. To $O(Y[\mathbf{n}]^2)$, we obtain the following RG flow equations[1]:

$$\partial_\ell (K_\ell^{-1})_{ab} = 2\pi^2 \sum_{\mathbf{n} \neq 0} n^a n^b Y[\mathbf{n}] Y[-\mathbf{n}] \quad (1)$$

$$\partial_\ell Y[\mathbf{n} \neq 0] = (2 - n^a K_{ab} n^b) Y[\mathbf{n}] + \sum_{\mathbf{n}' \neq 0, \mathbf{n}} \pi Y[\mathbf{n}'] Y[\mathbf{n} - \mathbf{n}'] \quad (2)$$

Equation(1) comes from the annihilation of dipoles of opposite vector charges in the annulus $a_0 < |r_i - r_j| < a_0 e^{d\ell}$. It gives the renormalisation of the interaction and of the disorder. Simple rescaling gives the first part of equation (2). The second part comes from the possibility of fusion of two replica vector charges upon coarse graining. Some examples of fusion are given below.

$$\begin{pmatrix} \vdots \\ +1 \\ \vdots \\ +1 \\ \vdots \\ 0 \\ \vdots \end{pmatrix} + \begin{pmatrix} \vdots \\ 0 \\ \vdots \\ 0 \\ \vdots \\ -1 \\ \vdots \end{pmatrix} \to \begin{pmatrix} \vdots \\ +1 \\ \vdots \\ +1 \\ \vdots \\ -1 \\ \vdots \end{pmatrix}, \begin{pmatrix} \vdots \\ +1 \\ \vdots \\ 0 \\ \vdots \\ 0 \\ \vdots \end{pmatrix} + \begin{pmatrix} \vdots \\ 0 \\ \vdots \\ +1 \\ \vdots \\ 0 \\ \vdots \end{pmatrix} \to \begin{pmatrix} \vdots \\ +1 \\ \vdots \\ +1 \\ \vdots \\ 0 \\ \vdots \end{pmatrix}, \begin{pmatrix} \vdots \\ +1 \\ \vdots \\ 0 \\ \vdots \\ 1 \\ \vdots \end{pmatrix} + \begin{pmatrix} \vdots \\ -1 \\ \vdots \\ 0 \\ \vdots \\ 0 \\ \vdots \end{pmatrix} \to \begin{pmatrix} \vdots \\ 0 \\ \vdots \\ 0 \\ \vdots \\ 1 \\ \vdots \end{pmatrix},$$

Replica permutation symmetry, which we will assume here and which is preserved by the RG, together with $n^a = 0, \pm 1$ implies that $Y[\mathbf{n}]$ depends only on the numbers $n_+$ and $n_-$ of $+1/-1$ components of $\mathbf{n}$. We parameterize $Y[\mathbf{n}]$ by introducing a function of two arguments $\Phi(z_+, z_-)$, where $z_\pm(\mathbf{r}) = \exp(\pm \beta v_\mathbf{r})$, such that:

$$Y[\mathbf{n}] = \langle z_+^{n_+} z_-^{n_-} \rangle_\Phi \quad (3)$$

where we denote $< A >_\Phi = \int dz_+ dz_- A \Phi(z_+, z_-)$. After some manipulations[1], in the limit $m \to 0$, we can write eq(2) in terms of, $P = \phi / (\int_{z_+, z_- > 0} \phi)$, which can be interpreted as a probability distribution, as

$$\partial_\ell P(z_+,z_-) = \mathcal{O}P - 2P(z_+,z_-) + 2\left\langle \delta\left(z_+ - \frac{z_+^{'}+z_+^{''}}{1+z_-^{'}z_+^{''}+z_+^{'}z_-^{''}}\right)\delta\left(z_- - \frac{z_-^{'}+z_-^{''}}{1+z_-^{'}z_+^{''}+z_+^{'}z_-^{''}}\right)\right\rangle_{P'P''}, \quad (4)$$

where, $\mathcal{O} = \beta E_C(2 + z_+\partial_{z_+} + z_-\partial_{z_-}) + \eta(\beta E_C)^2(z_+\partial_{z_+} - z_-\partial_{z_-})^2$. The $m \to 0$ limit of eq(1) similarly yields,

$$T\frac{dE_C^{-1}}{d\ell} = 8\left\langle \frac{z_+^{'}z_-^{''}+z_-^{'}z_+^{''}+4z_+^{'}z_-^{''}z_-^{'}z_+^{''}}{(1+z_+^{'}z_-^{''}+z_-^{'}z_+^{''})^2}\right\rangle_{PP} \quad (5)$$

$$\frac{d\eta}{d\ell} = 8\left\langle \frac{(z_+^{'}z_-^{''}-z_-^{'}z_+^{''})^2}{(1+z_+^{'}z_-^{''}+z_-^{'}z_+^{''})^2}\right\rangle_{PP} \quad (6)$$

Equations (4),(5) and (6) form the complete set of RG equations.

Numerical study[1] of the RG equations indicate the existence of an XY phase at low temperatures and below some critical disorder. Guided by the RG flow observed numerically within and near the boundaries of the XY phase, we can approximate the full RG equations by a simpler equation involving only the single fugacity distribution, $P_\ell(z) = \int dz_+ P_\ell(z_+, z) = \int dz_- P_\ell(z, z_-)$. In the low T regime, the distribution $P_\ell(z_+, z_-)$ is broad and the physics is dominated by rare favorable regions ($z_+ \sim 1$ or $z_- \sim 1$). Here we identify a parameter that allows to organise perturbation theory as: $P_\ell(1) \equiv P_\ell(z \sim 1) \sim P_\ell(z_+ \sim 1, z_- \sim 0) = P_\ell(z_+ \sim 0, z_- \sim 1)$We also observe that $P_\ell(1,1) \equiv P_\ell(z_+ \sim 1, z_- \sim 1) \sim P_\ell(1)^2$. Using these we can see schematically the RG equation (4) as a correction to $P_\ell(1)$ of order $P_\ell(1)$ by the first term and order $P_\ell(1)^2$ by the second term; in RG equation (5),(6) as a correction to order $P_\ell(1)^2$ to $(E_C)_\ell$ and $\eta_\ell$. Again working to order $P_\ell(1)^2$, we see that the denomenators in the delta functions in (4) could be neglected. This approximation also simplifies equations (5) and (6).

Introducing ,

$$G_\ell(x) = 1 - \int_{-\infty}^{\infty} du\tilde{P}_\ell(u)exp(-e^{\beta(u-x+E_\ell)}),, \quad (7)$$

where, $u = 1/\beta\ln(z)$ ,$E_\ell = \int_0^\ell E_C(\ell^{'})d\ell^{'}$ and the distribution $\tilde{P}(u)$ is defined as, $\tilde{P}(u)\mathrm{d}u = P(z)\mathrm{d}z$, we see that (4) can be written as $\frac{1}{2}\partial_\ell G = \frac{\eta E_C^2}{2}\partial_x^2 G + G(1-G)$. If $\eta$ and $E_C$ are $\ell$ independent we identify the above with Kolmogorov-Petrovskii-Piscounov (KPP) equation, whose general form is , $\frac{1}{2}\partial_\ell G = D\partial_x^2 G + f(G)$, where $D$ is a constant and $f$ satisfies $f(0) = f(1) = 0$, $f$ positive between 0 and 1 and $f^{'}(0) = 1, f^{'}(G) \leq 1$ between 0 and 1. Since at large $\ell$, both $E_C$ and $\eta$ converge and effectively becomes $\ell$ independent, we see that we can use results from the study of KPP equation in our case at large $\ell$.

For a large class of initial conditions, the solutions of the KPP equation are known to converge uniformly towards travelling wave solutions of the form: $G_\ell(x) \to h(x - m_\ell)$. The velocity of the wave is given by $c = \lim_{\ell\to\infty}\partial_\ell m_\ell$. A theorem due to Bramson[2] shows that the asymptotic travelling wave is determined by the behavior at $x \to \infty$ of the initial condition $G_{\ell=0}(x)$ in the following manner. If $G_{\ell=0}(x)$ decays faster than $e^{-\mu x}$ where $\mu = 1/\sqrt{D}$, then $c = \sqrt{D}$. If $G_{\ell=0}(x)$ decays slower than $e^{-\mu x}$ where $\mu = 1/\sqrt{D}$, then $c = 2(D\mu + \mu^{-1})$. The parameterisation(7) implies that the distribution $\tilde{P}_\ell(u)$ itself converges to a travelling front solution

$$\tilde{P}_\ell(u) \to_{\ell\to\infty} \tilde{p}(u - X_\ell)\ ,\ X_\ell = m_\ell - E_\ell. \quad (8)$$

Since $\partial_\ell E_\ell \to_{\ell\to\infty} (E_C)_R$, we see that the asymptotic velocity of the front of $\tilde{P}_\ell(u)$ is $c - (E_C)_R$, where $c$ is the KPP front velocity. $P_\ell(1)$ can be estimated crudely as $\tilde{p}(-X_\ell)$[3].

The asymptotic velocity clearly decides the phase of the system: since we start with a distribution peaked at some small $z$, if the velocity is positive, then $P_\ell(1)$ will increase and this would imply that the system is in the disordered phase. On the other hand negative velocity implies that the system is in the XY phase. The velocity vanishes at the phase boundary. By construction, the initial condition $G_{\ell=0}(x)$ decays for large $x$ as $< z >_{P_0} e^{-\beta x}$. Hence we identify $\mu = \beta$. Based on the results discussed above about the front velocity selection in KPP equation we can conclude the following about the phase diagram of the model:

(a) For $T > T_g = (E_C)_R\sqrt{\eta_R/2}$, $c = T\left(2 + \frac{\eta_R(E_C)_R^2}{T^2}\right)$. Thus here the XY phase would exist for

$$2 - \frac{(E_C)_R}{T} + \frac{\eta_R(E_C)_R^2}{T^2} < 0. \quad (9)$$

(b) For $T \leq T_g$, $c = (E_C)_R\sqrt{8\eta_R}$. Thus here the XY phase would exist for $\eta_R < \eta_c = \frac{1}{8}$.

*Critical behavior at zero temperature:* The zero temperature phase transition from the XY phase to the disordered phase occurs at $\eta_R = 1/8$. The centre of the front is located at $u = X_\ell$ near the transition. It follows from [2] that, $X_\ell \approx (4\sqrt{D} - E_C)\ell - 3/2\sqrt{D}\ln\ell + X_0$. Hence in the critical region to leading order, we get,

$$\partial_\ell X_\ell \sim 4\sqrt{D} - E_C - \frac{3\sqrt{D}}{2\ell}. \quad (10)$$

To estimate the form of correlation length, we first introduce the small parameter, $g_\ell = \exp(X_\ell/\sqrt{D})$. Then (10) reads

$$\partial_\ell g \sim \left(16(\eta - \eta_c) - \frac{3}{2l}\right) g$$

Now starting away from criticality, $\epsilon = \eta_c - \eta_R > 0$, we find, $g_\ell \sim \ell^{-3/2} \exp(16\epsilon\ell)$. Identifying the correlation length $\xi$ as when $g_\xi \sim 1$, we find

$$\xi \sim \exp\left(\frac{b}{|\eta - \eta_c|}\right),$$

where $b$ is some constant. We then see that the universality class of this transition is clearly different from the KT universlity class.

### B. Comparison with finite temperature insulator arising from many-body localization

Table I shows a comparison of the results of our analysis with the picture arising in the many body localization [4–6] approach.


[1] D. Carpentier and P. Le Doussal, Nuclear Physics B **588**, 565 (2000).
[2] M. Bramson, Memoirs of the American Mathematical Society **44**, 1 (1983).
[3] T. Giamarchi and H. J. Schulz, Physical Review B **37**, 325 (1988).
[4] I. V. Gornyi, A. D. Mirlin, and D. G. Polyakov, Phys. Rev. Lett. **95**, 2006603 (2005).
[5] D. M. Basko, I. L. Aleiner, and B. L. Altshuler, Annals of Physics **321**, 1126 (2006).
[6] S. Gopalakrishnan and R. Nandkishore, Phys. Rev. B **90**, 224203 (2012).
[7] L. Fleishman and P. W. Anderson, Physical Review B **21**, 2366 (1980).
[8] B. Altshuler, E. Cuevas, L. Ioffe, and V. Kravtsov, arXiv preprint arXiv:1605.02295 (2016).
[9] L.-H. Tang, Physical Review B **54**, 3350 (1996).
[10] B. Derrida and H. Spohn, Journal of Statistical Physics **51**, 817 (1988).

| Property | Quantum many-body localization | 2D disordered Coulomb gas |
| --- | --- | --- |
| Transport and critical behaviour | $\sigma(T) = \begin{cases} 0,\ T < T_{\mathrm{MBL}} \\ Ae^{-\sqrt{T_0/(T-T_{\mathrm{MBL}})}},\ T > T_{\mathrm{MBL}} \end{cases}$[4] | $\sigma(T) = 0$ in superinsulator phase, $\sigma(T) \sim \begin{cases} e^{-\sqrt{T_0/(T-T_{\mathrm{BKT}})}},\ T > T_{\mathrm{BKT}},\ \eta < \eta_c \\ e^{-A/(T-T_c)},\ \eta > \eta_c \end{cases}$ |
| Nature of interaction | Finite temperature insulator has been demonstrated for short range interactions. However long range interactions may drive $T_{\mathrm{MBL}}$ to zero.[7] | Logarithmic Coulomb interaction germane to finite temperature insulator. Further, VF scaling for $\sigma(T)$ requires logarithmically correlated disorder. |
| Mechanism | $\sigma(T) = 0$ if the gap in the spectrum of many-particle bath excitations exceeds the corresponding inelastic scattering rate.[4, 5] Finite $\sigma$ due to thermal activation above mobility edge not possible as mobility edge diverges with system volume.[5] | (a) Low disorder ($\eta \ll \eta_c$): Transition from superinsulator phase $\sigma(T) = 0$ occurs when long-range Coulomb interaction gets screened by thermally generated low-energy charge dipole excitations. (b) High disorder ($\eta > \eta_c$): Transition occurs due to seeding of low-energy single charge excitations due to deep potential fluctuations. |
| Erogodicity | MBL phase is nonergodic. Recent work[8] suggests existence of a nonergodic delocalized phase near the MBL phase, and also that the transition between the nonergodic and ergodic delocalized phases resembles the classical glass transition. | Phase diagram has both ergodic and nonergodic regions with respect to the occurence of charge dipoles. Dilute gas of dipoles freezes[9] for $T/E_c < \eta$. Transition from XY to conducting phase can take place in both the ergodic and nonergodic regions resulting in KT-like or VF-like scaling respectively for $\sigma(T)$. |
| Cayley tree structure | Transition temperature and critical behaviour are obtained by an approximate mapping of the problem to an Anderson model in Fock space with a Cayley tree structure. | Scaling equation for charge fugacity in the disordered model can be recast in the form of the KPP equation (see SI) in relevant variables. The KPP equation arises naturally in studies of directed polymers on the Cayley tree.[10] |

Table I: Comparison of two different theoretical routes to superinsulating behaviour based on (i) quantum many body localization and (ii) 2D disordered Coulomb gas (proposed in this paper).
